# Supplementary material for: The Spin-MInt Algorithm: an Accurate and Symplectic Propagator for the Spin-Mapping Representation of Nonadiabatic Dynamics
Source: arXiv:2512.01579 ancillary file (2026-03-12)
Supplement: Supplementary file 1 [file SI_Spin_MInt.pdf]

# Supplementary Material: The Spin-MInt Algorithm: an Accurate and Symplectic Propagator for the Spin-Mapping Representation of Nonadiabatic Dynamics

Lauren E. Cook,<sup>1</sup> James R. Rampton,<sup>1</sup> and Timothy J. H. Hele<sup>1, a)</sup>

*Department of Chemistry, University College London, Christopher Ingold Building,  
London WC1H 0AJ, United Kingdom*

(Dated: 30 November 2025)

The supplementary material comprises of three sections; additional algebra, three-state model and additional results. Additional algebra is listed in the table of contents. The three-state model section tabulates model parameters and details the sampling. Additional results includes single trajectories, ensemble conservation of spin-magnitude and energy, and tabulated code racing data.

## CONTENTS

|                                          |    |
|------------------------------------------|----|
| <b>I. Supplementary Algebra</b>          | 2  |
| A. Decomposition of $V$                  | 2  |
| B. Decomposition of $W$                  | 2  |
| C. Alternative Spin-MInt $P$ propagation | 3  |
| D. Explicit Monodromy Calculations       | 4  |
| E. Satisfaction of Liouville's Theorem   | 6  |
| F. Symplecticity Proof                   | 7  |
| G. Split-Liouvillian Spin Algorithm      | 9  |
| <b>II. Three State Model</b>             | 12 |
| <b>III. Supplementary Results</b>        | 13 |
| A. Single Trajectory                     | 13 |
| B. Ensemble                              | 18 |
| 1. Model 1                               | 18 |
| 2. Models 2 and 3                        | 19 |
| C. Code Racing                           | 21 |
| <b>References</b>                        | 23 |

---

<sup>a)</sup>Electronic mail: t.hele@ucl.ac.uk

## I. SUPPLEMENTARY ALGEBRA

### A. Decomposition of $\mathbf{V}$

The eigenvalues and eigenvectors that decompose  $\mathbf{V}$  when  $\Delta$  is real are

$$\mathbf{S} = \begin{bmatrix} \cos \alpha & -\sin \alpha \\ \sin \alpha & \cos \alpha \end{bmatrix}, \quad (\text{S.1})$$

where  $\tan(2\alpha) = 2\Delta/(V_1 - V_2)$  and therefore

$$\mathbf{\Lambda} = \mathbf{S}^T \mathbf{V} \mathbf{S}. \quad (\text{S.2})$$

To ensure the derivatives of the eigenvectors and eigenvalues are consistent and continuous, we use the numpy function `arctan2` to stay in the correct quadrant. The derivatives are,<sup>1</sup>

$$\Lambda'_{nm} = \begin{cases} (\mathbf{S}^T \mathbf{V}' \mathbf{S})_{nm} & n = m \\ 0 & n \neq m, \end{cases} \quad (\text{S.3})$$

where we use  $\mathbf{S}'^T \mathbf{S} + \mathbf{S}^T \mathbf{S}' = \mathbb{O}$ . By differentiating the angle

$$\frac{\partial \alpha}{\partial R} = \frac{1}{2} \cos^2(2\alpha) \left( \frac{2\Delta'}{V_1 - V_2} - \frac{2\Delta(V_1' - V_2')}{(V_1 - V_2)^2} \right), \quad (\text{S.4})$$

we can obtain the eigenvector derivatives as,

$$\mathbf{S}' = \begin{bmatrix} -\sin \alpha & -\cos \alpha \\ \cos \alpha & -\sin \alpha \end{bmatrix} \times \frac{\partial \alpha}{\partial R}. \quad (\text{S.5})$$

### B. Decomposition of $\mathbf{W}$

The eigenvalues and eigenvectors that decompose  $\mathbf{W}$  where  $\Delta$  is real such that  $H_y = 0$  are

$$\mathbf{S}_W = \frac{1}{\sqrt{2}} \begin{bmatrix} \cos(\zeta) & \sqrt{2} \sin(\zeta) & \cos(\zeta) \\ -i & 0 & i \\ -\sin(\zeta) & \sqrt{2} \cos(\zeta) & \sin(\zeta) \end{bmatrix}, \quad (\text{S.6})$$

where  $\tan(\zeta) = 2\Delta/(V_1 - V_2)$ , which is half of the angle for  $\mathbf{V}$ , and

$$\mathbf{\Lambda}_W = \begin{bmatrix} -\sqrt{(V_1 - V_2)^2 + (2\Delta)^2} & 0 & 0 \\ 0 & 0 & 0 \\ 0 & 0 & \sqrt{(V_1 - V_2)^2 + (2\Delta)^2} \end{bmatrix}, \quad (\text{S.7})$$

where the first and third eigenvalue are a  $\pm$  pair. The derivatives with respect to  $R$  are

$$\mathbf{\Lambda}'_W = \frac{1}{\sqrt{(V_1 - V_2)^2 + (2\Delta)^2}} \begin{bmatrix} -(V_1 - V_2)(V'_1 - V'_2) - 4\Delta\Delta' & 0 & 0 \\ 0 & 0 & 0 \\ 0 & 0 & (V_1 - V_2)(V'_1 - V'_2) + 4\Delta\Delta' \end{bmatrix}, \quad (\text{S.8})$$

and

$$\frac{\partial \zeta}{\partial R} = \cos^2(\zeta) \left( \frac{2\Delta'}{V_1 - V_2} - \frac{2\Delta(V'_1 - V'_2)}{(V_1 - V_2)^2} \right), \quad (\text{S.9})$$

such that

$$\mathbf{S}'_W = \frac{1}{\sqrt{2}} \begin{bmatrix} \sin(\zeta) & \sqrt{2}\cos(\zeta) & \sin(\zeta) \\ 0 & 0 & 0 \\ -\cos(\zeta) & \sqrt{2}\sin(\zeta) & \cos(\zeta) \end{bmatrix} \times \frac{\partial \zeta}{\partial R}. \quad (\text{S.10})$$

### C. Alternative Spin-MInt $P$ propagation

The Spin-MInt propagation of  $P$  in Eqn. (45) is equivalent to deriving the evolution from  $H_{2,\text{SM}}$  in the form,

$$H_{2,\text{SM}}(\mathbf{u}) = V_0(R) + \frac{1}{2} \text{Tr}[\mathbf{V}(\mathbf{C}(\mathbf{u}) + \mathbb{I})], \quad (\text{S.11})$$

where

$$\mathbf{C}(\mathbf{u}) = \begin{bmatrix} u_z & u_x - iu_y \\ u_x + iu_y & -u_z \end{bmatrix}, \quad (\text{S.12})$$

which is related to the  $\mathbf{C}(\mathbf{q}, \mathbf{p}) = (\mathbf{q} + i\mathbf{p}) \otimes (\mathbf{q} - i\mathbf{p})^T$  matrix which is commonly used in expressions of correlation functions in mapping variables.<sup>2,3</sup> For a two level system, the relation is

$$\mathbf{C}(\mathbf{q}, \mathbf{p}) = \mathbf{C}(\mathbf{u}) + 2r_s \mathbb{I}. \quad (\text{S.13})$$

The propagation of  $P$  is then

$$\dot{P} = -\mathbf{V}'_0(R) - \frac{1}{2} \text{Tr}[\mathbf{V}'(R)(\mathbf{C}(\mathbf{u}, t) + \mathbb{I})], \quad (\text{S.14})$$

where to use the MInt approach to evolving the  $\mathbf{V}'(R)$  matrix, we need to know the time-evolution of the  $\mathbf{C}(\mathbf{u})$  matrix. Using Eqn. (S.13) where  $r_s$  is a constant of integration and Eqn. (10) from the main manuscript we obtain

$$\mathbf{C}(\mathbf{u}, t) = e^{-i\mathbf{V}t} \mathbf{C}(\mathbf{q}, \mathbf{p}, 0) e^{i\mathbf{V}t} - 2r_s \mathbb{I} \quad (\text{S.15a})$$

$$= e^{-i\mathbf{V}t} \mathbf{C}(\mathbf{u}, 0) e^{i\mathbf{V}t}, \quad (\text{S.15b})$$

where the time-derivative can be described by the commutator

$$\frac{d}{dt} \mathbf{C}(\mathbf{u}) = i[\mathbf{C}(\mathbf{u}), \mathbf{V}], \quad (\text{S.16})$$

and  $\hbar = 1$  throughout. We can now express the propagation of  $P$  as

$$P(t + \Delta t) = P(t) - \int_0^{\Delta t} dt \left( \mathbf{V}'_0 + \frac{1}{2} \text{Tr}[e^{i\mathbf{V}t} \mathbf{V}' e^{-i\mathbf{V}t} \mathbf{C}(\mathbf{u}, 0)] + \frac{1}{2} \text{Tr}[\mathbf{V}'] \right), \quad (\text{S.17})$$

where the integral of the second term can be found as in the original MInt paper and outlined in Section II.A.2 of the main manuscript, specifically Eqns. (14-19). The propagation is therefore

$$P_{\text{SM}}(t + \Delta t) = P(t) - \Delta t \left( \mathbf{V}'_0 + \frac{1}{2} \text{Tr}[\mathbf{V}'] \right) - \frac{1}{2} \text{Tr}[(\mathbf{E} + i\mathbf{F}) \mathbf{C}(\mathbf{u}, 0)]. \quad (\text{S.18})$$

## D. Explicit Monodromy Calculations

The Spin-MInt monodromy matrix for  $H_{2,\text{SM}}$  can be defined as

$$\mathbf{M}_{\text{SM}, H_{2,\text{SM}}} = \begin{bmatrix} 1 & 0 & 0 & 0 \\ a & b & 0 & c \\ d & e & 1 & f \\ g & h & 0 & j \end{bmatrix}, \quad (\text{S.19})$$

where

$$a = \frac{u_x(\mathbf{Q}'_2 \mathbf{u}) - u_y(\mathbf{Q}'_1 \mathbf{u})}{u_x^2 + u_y^2}, \quad (\text{S.20a})$$

$$b = \frac{u_x(\mathbf{Q}_2 \mathbf{v}_2) - u_y(\mathbf{Q}_1 \mathbf{v}_2)}{u_x^2 + u_y^2}, \quad (\text{S.20b})$$

$$c = \frac{u_x(\mathbf{Q}_2 \mathbf{v}_1) - u_y(\mathbf{Q}_1 \mathbf{v}_1)}{u_x^2 + u_y^2}, \quad (\text{S.20c})$$

$$d = -\Delta t \left( V''_0 + \frac{1}{2} \text{Tr}(\mathbf{V}'') \right) - \frac{(V''_1 - V''_2)}{2} \bar{\mathbf{Q}}_3 \mathbf{u} - \frac{(V'_1 - V'_2)}{2} \bar{\mathbf{Q}}'_3 \mathbf{u}, \quad (\text{S.20d})$$

$$e = \frac{-(V'_1 - V'_2)}{2} \bar{\mathbf{Q}}_3 \mathbf{v}_2, \quad (\text{S.20e})$$

$$f = \frac{-(V'_1 - V'_2)}{2} \bar{\mathbf{Q}}_3 \mathbf{v}_1, \quad (\text{S.20f})$$

$$g = \frac{1}{2} \mathbf{Q}'_3 \mathbf{u}, \quad (\text{S.20g})$$

$$h = \frac{1}{2} \mathbf{Q}_3 \mathbf{v}_2, \quad (\text{S.20h})$$

$$j = \frac{1}{2} \mathbf{Q}_3 \mathbf{v}_1, \quad (\text{S.20i})$$

and  $u_x/u_y/u_z$  are at evolved time,  $\mathbf{u}/\mathbf{v}_1/\mathbf{v}_2$  are at initial time. We let  $\mathbf{Q} = e^{-i\mathbf{W}t}$  such that the subscript denotes the row of this matrix, the prime denotes the derivative with respect to  $R$  and, the bar denotes the integral with respect to time. This is equivalent to Eqns. (C.13) of the main manuscript where  $\bar{\mathbf{Q}} = \mathbf{S}_W \mathbf{R} \mathbf{S}_W^\dagger$  and where  $\Delta$  is real and independent of nuclear position.

To prove the symplecticity, it is desirable to have an explicit form of each element of  $\mathbf{Q}$ . We let  $x = \Delta t(V_2 - V_1)$  and  $y = 2(\Delta t)\Delta$ , and use the power series expansion

$$\begin{aligned} \mathbf{Q} = \mathbb{I} + \begin{bmatrix} 0 & x & 0 \\ -x & 0 & -y \\ 0 & y & 0 \end{bmatrix} + \frac{1}{2!} \begin{bmatrix} -x^2 & 0 & -xy \\ 0 & -x^2 - y^2 & 0 \\ -xy & 0 & -y^2 \end{bmatrix} \\ + \frac{1}{3!} \begin{bmatrix} 0 & -x^3 - xy^2 & 0 \\ x^3 + xy^2 & 0 & x^2y + y^3 \\ 0 & -x^2y - y^3 & 0 \end{bmatrix} + \dots \end{aligned} \quad (\text{S.21a})$$

$$= \mathbb{I} + \sum_{n=0}^{\infty} (-x^2 - y^2)^n \begin{bmatrix} \frac{-x^2}{(2n+2)!} & \frac{x}{(2n+1)!} & \frac{-xy}{(2n+2)!} \\ \frac{-x}{(2n+1)!} & \frac{-x^2 - y^2}{(2n+2)!} & \frac{-y}{(2n+1)!} \\ \frac{-xy}{(2n+2)!} & \frac{y}{(2n+1)!} & \frac{-y^2}{(2n+2)!} \end{bmatrix} \quad (\text{S.21b})$$

$$= \mathbb{I} + \sum_{n=0}^{\infty} \frac{(-1)^n \sqrt{x^2 + y^2}^{2n+2}}{x^2 + y^2} \begin{bmatrix} \frac{-x^2}{(2n+2)!} & \frac{x}{(2n+1)!} & \frac{-xy}{(2n+2)!} \\ \frac{-x}{(2n+1)!} & \frac{-x^2 - y^2}{(2n+2)!} & \frac{-y}{(2n+1)!} \\ \frac{-xy}{(2n+2)!} & \frac{y}{(2n+1)!} & \frac{-y^2}{(2n+2)!} \end{bmatrix} \quad (\text{S.21c})$$

$$= \begin{bmatrix} \frac{y^2 + x^2 \cos(\sqrt{x^2 + y^2})}{x^2 + y^2} & \frac{x \sin(\sqrt{x^2 + y^2})}{\sqrt{x^2 + y^2}} & \frac{xy \cos(\sqrt{x^2 + y^2}) - xy}{x^2 + y^2} \\ \frac{-x \sin(\sqrt{x^2 + y^2})}{\sqrt{x^2 + y^2}} & \cos(\sqrt{x^2 + y^2}) & \frac{-y \sin(\sqrt{x^2 + y^2})}{\sqrt{x^2 + y^2}} \\ \frac{xy \cos(\sqrt{x^2 + y^2}) - xy}{x^2 + y^2} & \frac{y \sin(\sqrt{x^2 + y^2})}{\sqrt{x^2 + y^2}} & \frac{x^2 + y^2 \cos(\sqrt{x^2 + y^2})}{x^2 + y^2} \end{bmatrix}. \quad (\text{S.21d})$$

We also require  $\mathbf{Q}'$ ,  $\bar{\mathbf{Q}}$  and  $\bar{\mathbf{Q}}'$ . In the case where  $\Delta$  is independent of nuclear position (as we

have here),  $\partial y/\partial R = 0$ . Therefore, abbreviating  $\cos\left(\sqrt{x^2+y^2}\right)$  and  $\sin\left(\sqrt{x^2+y^2}\right)$  as  $C$  and  $S$  respectively, the derivative is

$$\mathbf{Q}' = \begin{bmatrix} \frac{2xy^2 \frac{\partial x}{\partial R}(C-1)}{(x^2+y^2)^2} - \frac{x^3 \frac{\partial x}{\partial R} S}{\sqrt{x^2+y^2}^3} & \frac{x^2 \frac{\partial x}{\partial R} C}{x^2+y^2} + \frac{y^2 \frac{\partial x}{\partial R} S}{\sqrt{x^2+y^2}^3} & \frac{y \frac{\partial x}{\partial R}(y^2-x^2)(C-1)}{(x^2+y^2)^2} - \frac{x^2 y \frac{\partial x}{\partial R} S}{\sqrt{x^2+y^2}^3} \\ -\frac{x^2 \frac{\partial x}{\partial R} C}{x^2+y^2} - \frac{y^2 \frac{\partial x}{\partial R} S}{\sqrt{x^2+y^2}^3} & \frac{-x \frac{\partial x}{\partial R} S}{\sqrt{x^2+y^2}} & -\frac{xy \frac{\partial x}{\partial R} C}{x^2+y^2} + \frac{xy \frac{\partial x}{\partial R} S}{\sqrt{x^2+y^2}^3} \\ \frac{y \frac{\partial x}{\partial R}(y^2-x^2)(C-1)}{(x^2+y^2)^2} - \frac{x^2 y \frac{\partial x}{\partial R} S}{\sqrt{x^2+y^2}^3} & \frac{xy \frac{\partial x}{\partial R} C}{x^2+y^2} - \frac{xy \frac{\partial x}{\partial R} S}{\sqrt{x^2+y^2}^3} & \frac{-2xy^2 \frac{\partial x}{\partial R}(C-1)}{(x^2+y^2)^2} - \frac{xy^2 \frac{\partial x}{\partial R} S}{\sqrt{x^2+y^2}^3} \end{bmatrix}. \quad (\text{S.22})$$

As  $x$  and  $y$  are both first order with respect to  $\Delta t$ , we define time-independent variables  $\hat{x} = x/\Delta t$  and  $\hat{y} = y/\Delta t$  in order to make the time dependence explicit, and write  $C(t)$  and  $S(t)$  as  $\cos\left(\Delta t \sqrt{\hat{x}^2 + \hat{y}^2}\right)$  and  $\sin\left(\Delta t \sqrt{\hat{x}^2 + \hat{y}^2}\right)$  respectively.

The integral with respect to time is then

$$\bar{\mathbf{Q}} = \int_0^{\Delta t} \begin{bmatrix} \frac{\hat{y}^2 + \hat{x}^2 C(t)}{\hat{x}^2 + \hat{y}^2} & \frac{\hat{x} S(t)}{\sqrt{\hat{x}^2 + \hat{y}^2}} & \frac{\hat{x} \hat{y}(C(t)-1)}{\hat{x}^2 + \hat{y}^2} \\ \frac{-\hat{x} S(t)}{\sqrt{\hat{x}^2 + \hat{y}^2}} & C(t) & \frac{-\hat{y} S(t)}{\sqrt{\hat{x}^2 + \hat{y}^2}} \\ \frac{\hat{x} \hat{y}(C(t)-1)}{\hat{x}^2 + \hat{y}^2} & \frac{\hat{y} S(t)}{\sqrt{\hat{x}^2 + \hat{y}^2}} & \frac{\hat{x}^2 + \hat{y}^2 C(t)}{\hat{x}^2 + \hat{y}^2} \end{bmatrix} dt \quad (\text{S.23a})$$

$$= \Delta t \begin{bmatrix} \frac{y^2}{x^2+y^2} + \frac{x^2 S}{\sqrt{x^2+y^2}^3} & \frac{-x(C-1)}{x^2+y^2} & \frac{xy S}{\sqrt{x^2+y^2}^3} - \frac{xy}{x^2+y^2} \\ \frac{x(C-1)}{x^2+y^2} & \frac{S}{\sqrt{x^2+y^2}} & \frac{y(C-1)}{x^2+y^2} \\ \frac{xy S}{\sqrt{x^2+y^2}^3} - \frac{xy}{x^2+y^2} & \frac{-y(C-1)}{x^2+y^2} & \frac{x^2}{x^2+y^2} + \frac{y^2 S}{\sqrt{x^2+y^2}^3} \end{bmatrix}. \quad (\text{S.23b})$$

Differentiating this with respect to  $R$  results in,

$$\bar{\mathbf{Q}}' = \Delta t \frac{\partial x}{\partial R} \begin{bmatrix} \frac{x(x^2 C - 2y^2)}{(x^2+y^2)^2} + \frac{xS(2y^2-x^2)}{\sqrt{x^2+y^2}^5} & \frac{x^2 S}{\sqrt{x^2+y^2}^3} - \frac{y^2 C}{(x^2+y^2)^2} & \frac{y(x^2 C - y^2)}{(x^2+y^2)^2} + \frac{y(y^2 - 2x^2)S}{\sqrt{x^2+y^2}^5} \\ -\frac{x^2 S}{\sqrt{x^2+y^2}^3} + \frac{y^2 C}{(x^2+y^2)^2} & \frac{x C}{x^2+y^2} - \frac{x S}{\sqrt{x^2+y^2}^3} & \frac{-xy S}{\sqrt{x^2+y^2}^3} - \frac{2xy C}{(x^2+y^2)^2} \\ \frac{y(x^2 C - y^2)}{(x^2+y^2)^2} + \frac{y(y^2 - 2x^2)S}{\sqrt{x^2+y^2}^5} & \frac{xy S}{\sqrt{x^2+y^2}^3} + \frac{2xy C}{(x^2+y^2)^2} & \frac{xy^2(2+C)}{(x^2+y^2)^2} - \frac{3xy^2 S}{\sqrt{x^2+y^2}^5} \end{bmatrix}. \quad (\text{S.24})$$

We now use these forms to aid in algebraically determining symplecticity.

## E. Satisfaction of Liouville's Theorem

The determinant of  $\mathbf{M}_{\text{SM}, H_{2, \text{SM}}}$  is given by Eqn. (C.15) in the main manuscript, substituting the variables given in Eqn. (C.13), we obtain

$$|\mathbf{M}_{\text{SM}, H_{2, \text{SM}}}| = \frac{1}{2(u_x^2 + u_y^2)}(u_x(\kappa - \beta) + u_y(\varepsilon - \delta)), \quad (\text{S.25})$$

where  $u_x$ ,  $u_y$  and  $u_z$  are at time  $t$  and,

$$\kappa = (\mathbf{Q}_3 \cdot \mathbf{v}_1)(\mathbf{Q}_2 \cdot \mathbf{v}_2), \quad (\text{S.26a})$$

$$\beta = (\mathbf{Q}_2 \cdot \mathbf{v}_1)(\mathbf{Q}_3 \cdot \mathbf{v}_2), \quad (\text{S.26b})$$

$$\varepsilon = (\mathbf{Q}_1 \cdot \mathbf{v}_1)(\mathbf{Q}_3 \cdot \mathbf{v}_2), \quad (\text{S.26c})$$

$$\delta = (\mathbf{Q}_3 \cdot \mathbf{v}_1)(\mathbf{Q}_1 \cdot \mathbf{v}_2), \quad (\text{S.26d})$$

which are at time 0.

Expanding these using the expressions for the  $\mathbf{Q}$  in Eqn. (S.21) and  $\mathbf{v}$  in the main manuscript Eqn. (C.7), we find that  $(\kappa - \beta) = 2u_x$  and  $(\varepsilon - \delta) = 2u_y$ . It is useful to note that since the exponential matrix is an element of  $\text{SO}(3)$ , it is equal to its own cofactor matrix. This results in the following relations

$$Q_{ij} = \begin{cases} Q_{kk}Q_{ll} - Q_{kl}Q_{lk} & i = k \text{ and } k \neq l \neq i \\ Q_{ki}Q_{jk} - Q_{ji}Q_{kk} & i \neq j \text{ and } k \neq i, k \neq j, \end{cases} \quad (\text{S.27})$$

where  $Q_{ij}$  is the  $j$ th element of the row vector  $\mathbf{Q}_i$ . Hence,  $|\mathbf{M}_{\text{SM}, H_{2, \text{SM}}}| = 1$  as required for satisfaction of Liouville's theorem.

## F. Symplecticity Proof

We recall that in Eqn. (C.16), in order to prove symplecticity we wish to show that

$$C_1 = bg - e - ah = 0, \quad (\text{S.28a})$$

$$C_2 = cg - f - aj = 0. \quad (\text{S.28b})$$

Using the cofactor relations Eqn. (S.27),

$$(\mathbf{Q}_1 \mathbf{u})(\mathbf{Q}_2 \mathbf{v}_2) - (\mathbf{Q}_1 \mathbf{v}_2)(\mathbf{Q}_2 \mathbf{u}) = \frac{4r_s^2 \sin^2 \theta}{2} (\mathbf{Q}_3 \mathbf{v}_1) \quad (\text{S.29})$$

$$(\mathbf{Q}_1 \mathbf{u})(\mathbf{Q}_2 \mathbf{v}_1) - (\mathbf{Q}_1 \mathbf{v}_1)(\mathbf{Q}_2 \mathbf{u}) = \frac{-2}{\sin^2 \theta} (\mathbf{Q}_3 \mathbf{v}_2), \quad (\text{S.30})$$

such that we can rewrite  $b$  and  $c$

$$b = 2r_s^2 \sin^2 \theta \frac{\mathbf{Q}_3 \mathbf{v}_1}{u_x^2 + u_y^2}, \quad (\text{S.31})$$

$$c = \frac{-2}{\sin^2 \theta} \frac{\mathbf{Q}_3 \mathbf{v}_2}{u_x^2 + u_y^2}, \quad (\text{S.32})$$

and Eqns. (S.28) become

$$C_1 = \frac{V'_2 - V'_1}{2} \bar{\mathbf{Q}}_3 \mathbf{v}_1 + \frac{\mathbf{Q}_3 \mathbf{v}_1 (u_x(\mathbf{Q}'_2 \mathbf{u}) - u_y(\mathbf{Q}'_1 \mathbf{u}))}{2(u_x^2 + u_y^2)} + \frac{(\mathbf{Q}_3 \mathbf{v}_2)(\mathbf{Q}'_3 \mathbf{u})}{\sin^2 \theta (u_x^2 + u_y^2)}, \quad (\text{S.33a})$$

$$C_2 = \frac{V'_2 - V'_1}{2} \bar{\mathbf{Q}}_3 \mathbf{v}_2 + \frac{\mathbf{Q}_3 \mathbf{v}_2 (u_x(\mathbf{Q}'_2 \mathbf{u}) - u_y(\mathbf{Q}'_1 \mathbf{u}))}{2(u_x^2 + u_y^2)} - \frac{r_s^2 \sin^2 \theta (\mathbf{Q}_3 \mathbf{v}_1)(\mathbf{Q}'_3 \mathbf{u})}{(u_x^2 + u_y^2)}. \quad (\text{S.33b})$$

We note that these two criteria are equivalent using the identity  $\mathbf{Q}'_3 \mathbf{u} = \frac{V'_1 - V'_2}{2} ((\bar{\mathbf{Q}}_3 \mathbf{v}_1)(\mathbf{Q}_3 \mathbf{v}_2) - (\mathbf{Q}_3 \mathbf{v}_1)(\bar{\mathbf{Q}}_3 \mathbf{v}_2))$ , such that satisfaction of one directly leads to satisfaction of the other. We first rearrange (S.33b),

$$\mathbf{Q}_3 \mathbf{v}_2 ((\mathbf{Q}_1 \mathbf{u})(\mathbf{Q}'_2 \mathbf{u}) - (\mathbf{Q}_2 \mathbf{u})(\mathbf{Q}'_1 \mathbf{u})) = (V'_1 - V'_2) (\bar{\mathbf{Q}}_3 \mathbf{v}_2) (u_x^2 + u_y^2) + 2r_s^2 \sin^2 \theta (\mathbf{Q}_3 \mathbf{v}_1)(\mathbf{Q}'_3 \mathbf{u}), \quad (\text{S.34})$$

and use the previously stated identity, collecting terms with a factor  $\bar{\mathbf{Q}}_3 \mathbf{v}_2$  on the right hand side (RHS), we may rewrite the RHS as

$$(V'_1 - V'_2) \left( (\bar{\mathbf{Q}}_3 \mathbf{v}_2) \left( u_x^2 + u_y^2 - (\mathbf{Q}_3 \mathbf{v}_1 r_s \sin \theta)^2 \right) + (\mathbf{Q}_3 \mathbf{v}_1 r_s \sin \theta) (\bar{\mathbf{Q}}_3 \mathbf{v}_1 r_s \sin \theta) (\mathbf{Q}_3 \mathbf{v}_2) \right). \quad (\text{S.35})$$

As  $u_x^2 + u_y^2 = 4r_s^2 - u_z^2$ , it can be verified that  $4r_s^2 - u_z^2 - (\mathbf{Q}_3 \mathbf{v}_1 r_s \sin \theta)^2 = (\mathbf{Q}_3 \mathbf{v}_2 / \sin \theta)^2$ . Thus cancelling  $\mathbf{Q}_3 \mathbf{v}_2$  from both sides

$$(\mathbf{Q}_1 \mathbf{u})(\mathbf{Q}'_2 \mathbf{u}) - (\mathbf{Q}_2 \mathbf{u})(\mathbf{Q}'_1 \mathbf{u}) = (V'_1 - V'_2) \left( \frac{\bar{\mathbf{Q}}_3 \mathbf{v}_2}{\sin \theta} \frac{\mathbf{Q}_3 \mathbf{v}_2}{\sin \theta} + (\mathbf{Q}_3 \mathbf{v}_1 r_s \sin \theta) (\bar{\mathbf{Q}}_3 \mathbf{v}_1 r_s \sin \theta) \right). \quad (\text{S.36})$$

From here, one can carefully expand both sides, and compare the prefactors of the various combinations of  $\sin \theta$ ,  $\sin \phi$ ,  $\cos \theta$  and  $\cos \phi$  that arise. To compare likewise terms, we rearrange these using  $\sin^2 \theta + \cos^2 \theta = 1$  and the same for  $\phi$  such that the only remaining terms on both the LHS and RHS are those in  $\sin^2 \theta \cos^2 \phi$ ,  $\sin^2 \theta \cos \phi \sin \phi$ ,  $\cos \theta \sin \theta \cos \phi$ ,  $\cos \theta \sin \theta \sin \phi$ ,  $\sin^2 \theta$  and constant terms. This comparison is shown in Table S.1.

One can show that both the LHS and RHS expressions are equal to the explicit monodromy expressions, therefore  $C_1 = C_2 = 0$  and the propagation of  $H_{2,\text{SM}}$  is symplectic. As the propagation of  $H_{1,\text{SM}}$  is identical to the MInt and symplectic, overall the Spin-MInt algorithm is symplectic.

TABLE S.1. The prefactors of each remaining term in the LHS and RHS of (S.36), which are individually equal to the explicit monodromy expression, such Eqn. (S.36) is satisfied. Each side is divided by  $4r_s^2(V_2' - V_1')\Delta t$  to reduce the number of symbols, such that derivatives are divided by  $\partial x/\partial R$  and integrals by  $\Delta t$ .

| Term                                | LHS                                                             | RHS                                       | Explicit Monodromy                                                                   |
|-------------------------------------|-----------------------------------------------------------------|-------------------------------------------|--------------------------------------------------------------------------------------|
| $\sin^2 \theta \cos^2 \phi$         | $Q'_{21}(Q_{11} - Q_{22}) + Q_{21}(Q'_{22} - Q'_{11})$          | $\bar{Q}_{31}Q_{31} - \bar{Q}_{32}Q_{32}$ | $\frac{x^2y^2(1-C)}{(x^2+y^2)^2} + \frac{y^2(2x^2+y^2)S(C-1)}{\sqrt{x^2+y^2}^5}$     |
| $\sin^2 \theta \cos \phi \sin \phi$ | $Q'_{22}Q_{11} - Q'_{11}Q_{22}$                                 | $\bar{Q}_{31}Q_{32} + \bar{Q}_{32}Q_{31}$ | $\frac{2xy^2(C-C^2)}{(x^2+y^2)^2} - \frac{xy^2S}{\sqrt{x^2+y^2}^3}$                  |
| $\cos \theta \sin \theta \cos \phi$ | $Q'_{23}Q_{11} + Q'_{21}Q_{13} - Q'_{11}Q_{23} - Q'_{13}Q_{21}$ | $\bar{Q}_{31}Q_{33} + \bar{Q}_{33}Q_{31}$ | $\frac{-2x^3y}{(x^2+y^2)^2} + \frac{xy^3S(2C-1)+x^3yS}{\sqrt{x^2+y^2}^5}$            |
| $\cos \theta \sin \theta \sin \phi$ | $Q'_{23}Q_{12} + Q'_{22}Q_{13} - Q'_{12}Q_{23} - Q'_{13}Q_{22}$ | $\bar{Q}_{32}Q_{33} + \bar{Q}_{33}Q_{32}$ | $\frac{x^2y(1-C)+y^3(S^2+C-C^2)}{(x^2+y^2)^2} + \frac{x^2yS}{\sqrt{x^2+y^2}^3}$      |
| $\sin^2 \theta$                     | $Q'_{22}Q_{12} - Q'_{23}Q_{13} + Q'_{13}Q_{23} - Q'_{12}Q_{22}$ | $\bar{Q}_{32}Q_{32} - \bar{Q}_{33}Q_{33}$ | $\frac{-x^2(x^2+y^2C)}{(x^2+y^2)^2} + \frac{y^2S(y^2-x^2C-2y^2C)}{\sqrt{x^2+y^2}^5}$ |
| constant                            | $Q'_{23}Q_{13} - Q'_{13}Q_{23}$                                 | $\bar{Q}_{31}Q_{31} + \bar{Q}_{32}Q_{32}$ | $\frac{x^2y^2(C-1)}{(x^2+y^2)^2} + \frac{y^4S(C-1)}{\sqrt{x^2+y^2}^5}$               |

## G. Split-Liouvillian Spin Algorithm

One can derive a Split-Liouvillian (Spin-SL) algorithm for spin-mapping by using a Suzuki-Trotter decomposition. Despite previous claims that this will make the algorithm symplectic,<sup>4-6</sup> we can algebraically show that this form does not result in a symplectic algorithm when considering a non-trivial coupling between the electronic and nuclear DoF. This is as further splitting the Liouvillian for the sub-Hamiltonian  $H_2$  does not result in exact sub-Hamiltonian evolution,<sup>7</sup> and the energy will drift during simulation.<sup>8,9</sup> This is in agreement with previous work that found the SL algorithm for the MMST mapping to not be symplectic for the same reason.<sup>1,9</sup>

We can define the Liouvillian for  $H_{2,SM}$  in canonical variables as

$$\mathcal{L}_2 = \dot{P} \frac{\partial}{\partial P} + \dot{\phi} \frac{\partial}{\partial \phi} + r \cos \theta \frac{\partial}{\partial r \cos \theta}, \quad (\text{S.37})$$

which we can further split into

$$\mathcal{L}_P = \dot{P} \frac{\partial}{\partial P}, \quad (\text{S.38a})$$

$$\mathcal{L}_{el} = \dot{\phi} \frac{\partial}{\partial \phi} + r \cos \theta \frac{\partial}{\partial r \cos \theta}, \quad (\text{S.38b})$$

such that the evolution is

$$\Psi_{H_{SM}, \Delta t}^{\text{SL-Spin}} := e^{\mathcal{L}_{el} \frac{\Delta t}{2}} e^{\mathcal{L}_P \frac{\Delta t}{2}} e^{\mathcal{L}_1 \Delta t} e^{\mathcal{L}_P \frac{\Delta t}{2}} e^{\mathcal{L}_{el} \frac{\Delta t}{2}}, \quad (\text{S.39})$$

where a Suzuki-Trotter decomposition is used<sup>1,4,6,9</sup> and  $L_1$  is the Liouvillian for  $H_1$  resulting in the same nuclear position propagation as in the MInt and Spin-MInt algorithms. The corresponding flowmap is,

$$\Psi_{H_{SL}, \Delta t}^{\text{SL-Spin}} := \Psi_{\text{SL-Spin}^b, \frac{\Delta t}{2}} \circ \Phi_{H_1, \Delta t} \circ \Psi_{\text{SL-Spin}^a, \frac{\Delta t}{2}}, \quad (\text{S.40})$$

where  $\Psi_{\text{SL-Spin}^{a/b}}$  represents the approximate propagation of  $H_2$ . We have used a symmetric splitting such that the two half timesteps are not equal and the superscripts  $a$  is  $e^{-\mathcal{L}_P}e^{-\mathcal{L}_{\text{el}}}$  and  $b$  is  $e^{\mathcal{L}_{\text{el}}}e^{\mathcal{L}_P}$ . The EOM for  $H_{2,\text{SM}}$  are then,

$$\dot{P} = -V'_0(R) - \frac{1}{2}(\text{Tr}[\mathbf{V}'(R)] + \mathbf{H}'\mathbf{u}), \quad (\text{S.41a})$$

$$r\dot{\cos\theta} = \frac{1}{2}(H_x u_y - H_y u_x), \quad (\text{S.41b})$$

$$\dot{\phi} = H_z - H_x \frac{\cos\phi}{\tan\theta} - H_y \frac{\sin\phi}{\tan\theta}, \quad (\text{S.41c})$$

where the electronic EOM are easily shown to be equivalent to<sup>10,11</sup>

$$\dot{\mathbf{u}} = \mathbf{H} \times \mathbf{u}, \quad (\text{S.42})$$

and we can exactly integrate in the same way as for the Spin-MInt

$$\mathbf{u}(\Delta t/2) = e^{-i\mathbf{W}\Delta t/2}\mathbf{u}(0), \quad (\text{S.43})$$

for half a timestep. As the electronic evolution is identical to the Spin-MInt, this algorithm will be structure preserving but not necessarily symplectic.

The nuclear momentum can be integrated as

$$P(\Delta t/2) = P(0) - \frac{\Delta t}{2}(V'_0(R) + \frac{1}{2}(\text{Tr}[\mathbf{V}'(R)] + \mathbf{H}'\mathbf{u}(\Delta t/2))), \quad (\text{S.44})$$

where the electronic variables are the half timestep evolved values.

We can now test these EOM for symplecticity using the canonical variable monodromy matrix, Eqn (50) in the main manuscript and the symplecticity criterion

$$\mathbf{M}^T \mathbf{J}^{-1} \mathbf{M} = \mathbf{J}^{-1}, \quad (\text{S.45})$$

where  $J$  is the structure matrix outlined in Eqn. (49) of the main manuscript. We note that the propagation of  $H_1$  is symplectic such that we only need to test the propagation of  $H_2$ .

For the electronic evolution

$$\mathbf{M}_{\text{el}} = \begin{bmatrix} 1 & 0 & 0 & 0 \\ a & b & 0 & c \\ 0 & 0 & 1 & 0 \\ g & h & 0 & j \end{bmatrix}, \quad (\text{S.46})$$

where the elements are the same as for the Spin-MInt where  $\mathbf{u}$  is half timestep evolved and  $|\mathbf{M}_{\text{el}}| = 1$  as for the Spin-MInt. Evaluating the symplecticity results in

$$\mathbf{M}_{\text{el}}^T \mathbf{J}^{-1} \mathbf{M}_{\text{el}} = \begin{bmatrix} 0 & bg - ah & -1 & cg - aj \\ -bg + ah & 0 & 0 & -1 \\ 1 & 0 & 0 & 0 \\ -cg + ja & 1 & 0 & 0 \end{bmatrix}, \quad (\text{S.47})$$

which will be symplectic if  $bg - ah = 0$  and  $cg - ja$ . For the Spin-MInt, the symplecticity conditions in Eqn. (S.28) are satisfied such that the SL-Spin algorithm is not symplectic for a nuclear-dependent potential.

For the nuclear momentum

$$\mathbf{M}_P = \begin{bmatrix} 1 & 0 & 0 & 0 \\ 0 & 1 & 0 & 0 \\ \tilde{d} & \tilde{e} & 1 & \tilde{f} \\ 0 & 0 & 0 & 1 \end{bmatrix}, \quad (\text{S.48})$$

where,

$$\tilde{d} = -\frac{\Delta t}{2}(\mathbf{V}_0'' + \frac{1}{2}(\text{Tr}[\mathbf{V}''] + \mathbf{H}''\mathbf{u}(\Delta t/2))), \quad (\text{S.49a})$$

$$\tilde{e} = -\frac{\Delta t}{4}\mathbf{H}'\mathbf{v}_2(\Delta t/2), \quad (\text{S.49b})$$

$$\tilde{f} = -\frac{\Delta t}{4}\mathbf{H}'\mathbf{v}_1(\Delta t/2), \quad (\text{S.49c})$$

and it is easy to see  $|\mathbf{M}_P| = 1$ . Evaluating symplecticity results in

$$\mathbf{M}_P^T \mathbf{J}^{-1} \mathbf{M}_P = \begin{bmatrix} 0 & -\tilde{e} & -1 & -\tilde{f} \\ \tilde{e} & 0 & 0 & -1 \\ 1 & 0 & 0 & 0 \\ \tilde{f} & 1 & 0 & 0 \end{bmatrix}, \quad (\text{S.50})$$

which will be symplectic if  $\tilde{e} = \tilde{f} = 0$  which, as in the last case, will only be satisfied if there is no nuclear dependence of the potential matrix.

The combination of the two matrices is

$$\mathbf{M}_{\text{el}}\mathbf{M}_P = \begin{bmatrix} 1 & 0 & 0 & 0 \\ a & b & 0 & c \\ \tilde{d} & \tilde{e} & 1 & \tilde{f} \\ g & h & 0 & j \end{bmatrix}, \quad (\text{S.51})$$

which comparing to Eqn. (S.19) will only be symplectic if  $e = \tilde{e}$  and  $f = \tilde{f}$  which is only true in the trivial cases of all eigenvalues of  $\mathbf{W}$  being 0 or if there is no nuclear dependence of the potential matrix.

Therefore, the SL-Spin algorithm will not be symplectic as  $\mathbf{M}_{\text{el}}$ ,  $\mathbf{M}_P$  and the combination of  $\mathbf{M}_{\text{el}}\mathbf{M}_P$  are not symplectic. However, it will satisfy phase-space preservation through Liouville's theorem and due to the same electronic propagation as the Spin-MInt will preserve the Poisson structure. Hence, structure preservation or Suzuki-Trotter decomposition will not automatically lead to a symplectic algorithm when the Hamiltonian is coupled in a way that splitting the Liou-villian results in a loss of exact sub-Hamiltonian evolution.

## II. THREE STATE MODEL

Here, we tabulate the parameters for the three state Morse potential used in the main manuscript Figure 7. There are three models (A,B and C) from the literature.<sup>11,12</sup>

We focus the initial sampling on the first state by using action-angle variables

$$X_n = \sqrt{2J_n + \gamma} \sin \theta_n, \quad (\text{S.52})$$

$$P_n = \sqrt{2J_n + \gamma} \cos \theta_n, \quad (\text{S.53})$$

where  $\gamma = 2(r_s - 1)/N$ ,  $r_s = \sqrt{N+1}$  and

$$J_n = \begin{cases} 1 & n = 1 \\ 0 & n \neq 1, \end{cases} \quad (\text{S.54})$$

and  $\theta_n$  is uniformly sampled from  $[0, 2\pi]$ . We convert these MMST variables into spin-mapping variables to run the Spin-MInt trajectories.

TABLE S.2. The three state Morse potential parameters for Models A, B and C in atomic units. We have tabulated the values from Ref. [12] but included the model labels from both Refs. [11,12].

| Parameter     | A     |       |       | B     |       |       | C     |       |       |
|---------------|-------|-------|-------|-------|-------|-------|-------|-------|-------|
| Ref. [12]     | III   |       |       | II    |       |       | I     |       |       |
| Ref. [11]     | IA    |       |       | IB    |       |       | IC    |       |       |
| $i$           | 1     | 2     | 3     | 1     | 2     | 3     | 1     | 2     | 3     |
| $D_{ii}$      | 0.02  | 0.02  | 0.003 | 0.02  | 0.01  | 0.003 | 0.003 | 0.004 | 0.003 |
| $\alpha_{ii}$ | 0.40  | 0.65  | 0.65  | 0.65  | 0.40  | 0.65  | 0.65  | 0.6   | 0.65  |
| $R_{ii}$      | 4.0   | 4.5   | 6.0   | 4.5   | 4.0   | 4.4   | 5.0   | 4.0   | 6.0   |
| $c_{ii}$      | 0.02  | 0     | 0.02  | 0     | 0.01  | 0.02  | 0     | 0.01  | 0.006 |
| $ij$          | 12    | 13    | 23    | 12    | 13    | 23    | 12    | 13    | 23    |
| $A_{ij}$      | 0.005 | 0.005 | 0     | 0.005 | 0.005 | 0     | 0.002 | 0     | 0.002 |
| $\alpha_{ij}$ | 32    | 32    | 0     | 32    | 32    | 0     | 16    | 0     | 16    |
| $R_{ij}$      | 3.4   | 4.97  | 0     | 3.66  | 3.34  | 0     | 3.4   | 0     | 4.8   |
| $R_0$         | 2.1   |       |       | 3.3   |       |       | 2.9   |       |       |

For the nuclear sampling, we sample

$$\rho_{\text{nuclear}} = \frac{1}{\pi} e^{-(R-R_0)/(m\omega) - m\omega(P-P_0)}, \quad (\text{S.55})$$

where  $m = 20000$ ,  $\omega = 0.005$ ,  $P_0 = 0$  for all three models and,  $R_0$  is tabulated.

### III. SUPPLEMENTARY RESULTS

#### A. Single Trajectory

For the single trajectory tested in the main manuscript Figure 2, we present the nuclear (Figure. S.1) and electronic variable (Figure S.2) propagation for the  $\Delta t = 0.1$  timestep tested with Model 1. We additionally plot the  $\Delta t = 0.001$  results for the MInt algorithm in black to emphasise the fact that the MInt (cyan) and Spin-MInt (purple) are accurate at the coarser timestep.

For the nuclear variables, we see that there is only a slight deviation in the trajectories when using the angle-based algorithm (orange). However, the discrepancy is more obvious in the electronic variables where  $u_x$  deviates first which causes  $u_y$  and  $u_z$  to become slightly out of phase.

As Model 1 is near the adiabatic limit, the angle-based trajectories are more accurate than with Models 2 (Figures S.3 and S.4) and 3 (Figures S.5 and S.6) likely due to the strong coupling.

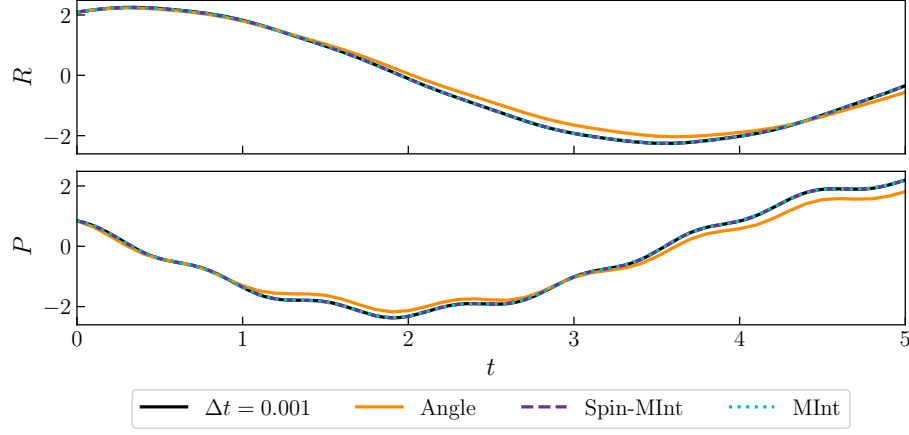

FIG. S.1. The nuclear position and momentum for the single trajectory in Figure 2 of the main manuscript for  $\Delta t = 0.1$ . The Spin-MInt (dotted purple) and MInt (dotted cyan) are in agreement with the MInt  $\Delta t = 0.001$  (black) results whilst the angle-based algorithm (orange) deviates.

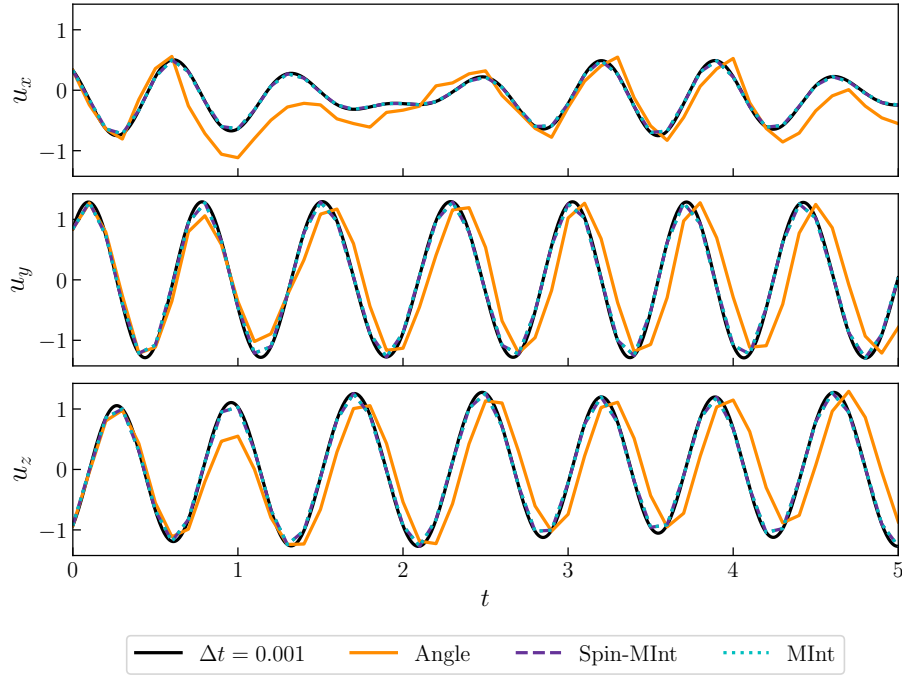

FIG. S.2. The electronic spin-mapping variables for the single trajectory in Figure 2 of the main manuscript for  $\Delta t = 0.1$ . The Spin-MInt (dotted purple) and MInt (dotted cyan) are in agreement with the MInt  $\Delta t = 0.001$  (black) results where the angle-based algorithm (orange) deviates with the largest deviation in  $u_x$ .

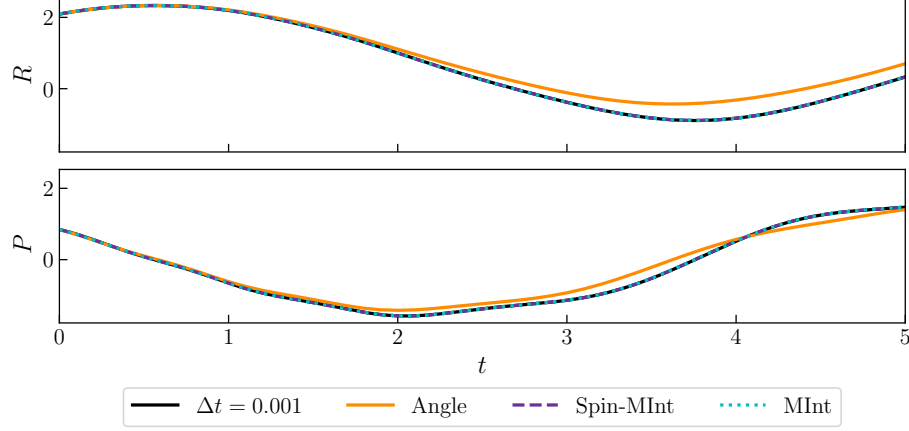

FIG. S.3. The nuclear position and momentum for a single trajectory using Model 2 with  $\Delta t = 0.1$ . The Spin-MInt (dotted purple) and MInt (dotted cyan) are in agreement with the MInt  $\Delta t = 0.001$  (black) results whilst the angle-based algorithm (orange) deviates.

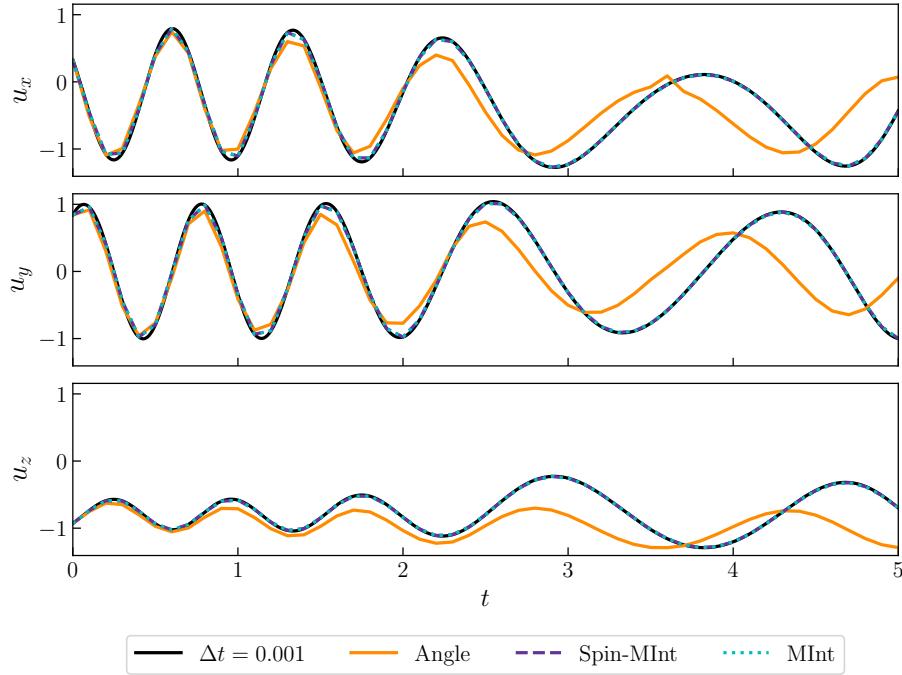

FIG. S.4. The electronic spin-mapping variables a single trajectory using Model 3 with  $\Delta t = 0.1$ . The Spin-MInt (dotted purple) and MInt (dotted cyan) are in agreement with the MInt  $\Delta t = 0.001$  (black) results where the angle-based algorithm (orange) deviates.

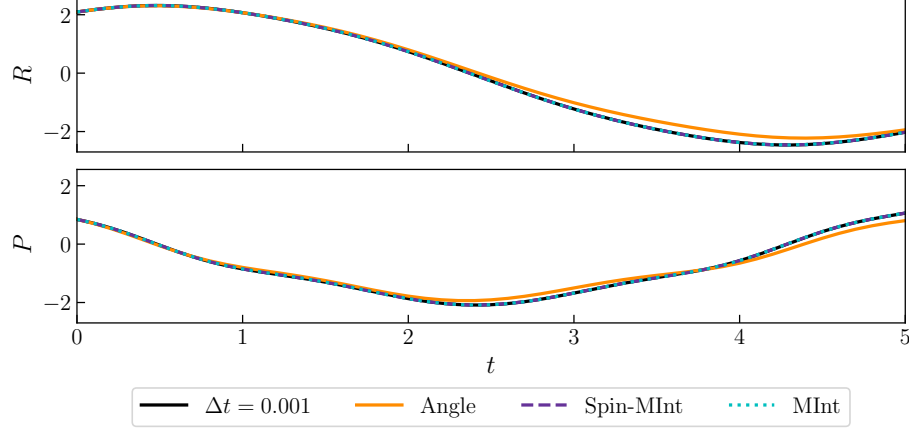

FIG. S.5. The nuclear position and momentum for a single trajectory using Model 3 with  $\Delta t = 0.1$ . The Spin-MInt (dotted purple) and MInt (dotted cyan) are in agreement with the MInt  $\Delta t = 0.001$  (black) results whilst the angle-based algorithm (orange) deviates.

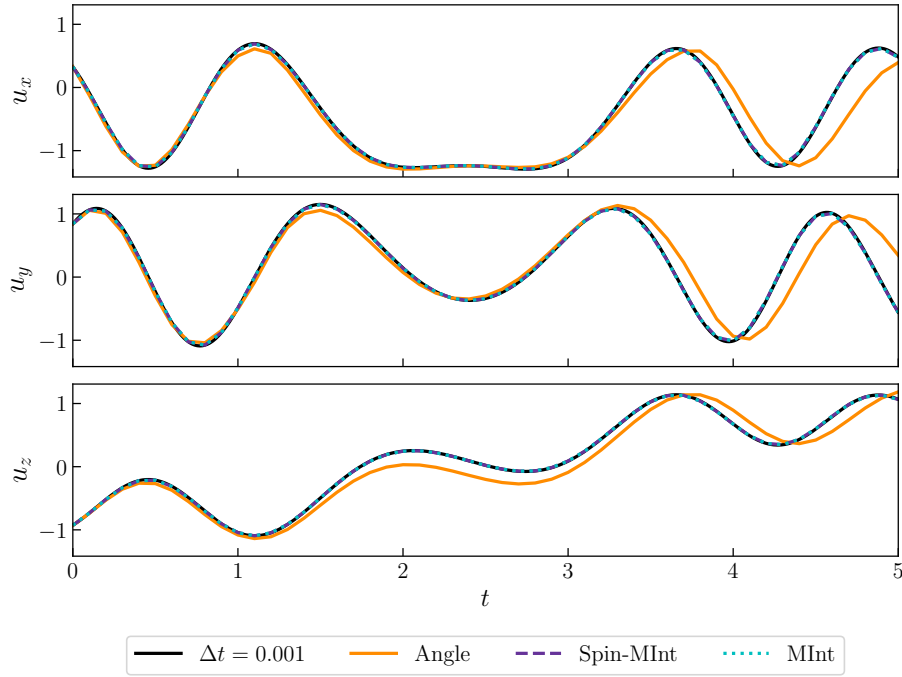

FIG. S.6. The electronic spin-mapping variables for a single trajectory using Model 3 with  $\Delta t = 0.1$ . The Spin-MInt (dotted purple) and MInt (dotted cyan) are in agreement with the MInt  $\Delta t = 0.001$  (black) results where the angle-based algorithm (orange) deviates.

Therefore, the angle-based algorithm is not as accurate as the Spin-MInt and MInt algorithms which are identical in propagation.

We then plot the symplecticity criterion by tracking the Frobenius norm of the error matrix,  $\mathbf{E}_r$ , defined in Eqn. (59) of the main manuscript. In Figure S.7, we plot three different timesteps  $\Delta t = 0.1$  (dashed),  $\Delta t = 0.01$  (solid),  $\Delta t = 0.001$  (dotted) to determine the order of the symplecticity satisfaction. We see that both the Spin-MInt (purple) and MInt (cyan) are symplectic at all timesteps tested. For a symplectic algorithm, the conservation will appear slightly worse at smaller timesteps due to more opportunity for floating point errors to build up.<sup>9</sup> The angle-based algorithm (orange) is not symplectic and is zero-order with respect to timestep as this does not change with smaller timesteps. This means that the symplecticity will not improve with smaller timesteps.<sup>9</sup>

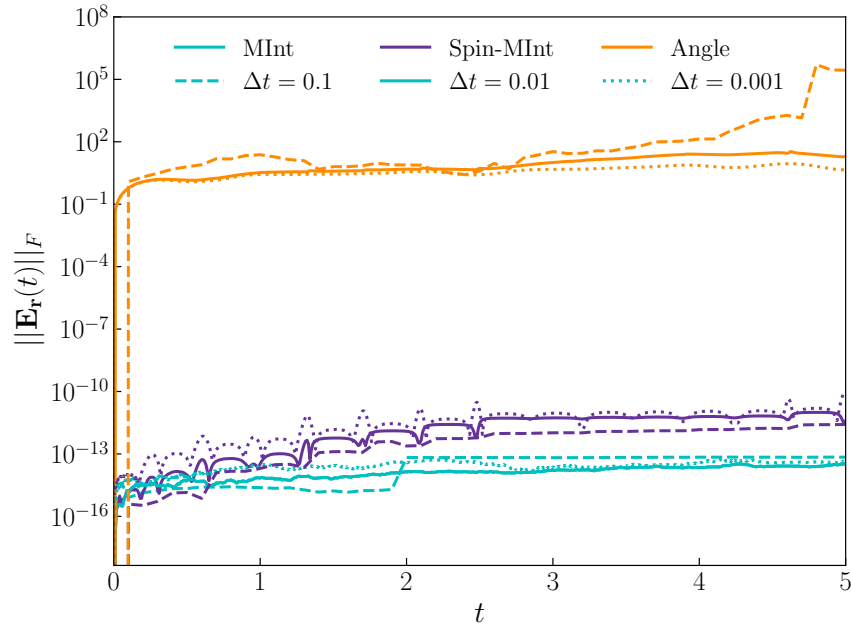

FIG. S.7. The error matrix Frobenius norm against time using Model 1 for a single trajectory and three timesteps  $\Delta t = 0.1$  (dashed),  $\Delta t = 0.01$  (solid),  $\Delta t = 0.001$  (dotted), using the Spin-MInt (purple), MInt (cyan) and angle-based (orange) algorithms. We see all algorithms are zero-order with respect to timestep and whilst the Spin-MInt and MInt algorithms are symplectic the angle-based algorithm is not.

We also track the symplecticity of the explicit monodromy matrix for the Spin-MInt algorithm outlined in Section ID. We plot this in Figure S.8 as a dashed purple line. We see a lower build-up of floating point errors when using this matrix compared to the generalised form seen in the main manuscript (purple solid) due to fewer calculations required. However, the explicit form of  $\mathbf{Q}$  is challenging to obtain for two electronic states,  $N = 2$ , we focus on the generalised form in the main manuscript as this can be easily computed for  $N > 2$ .

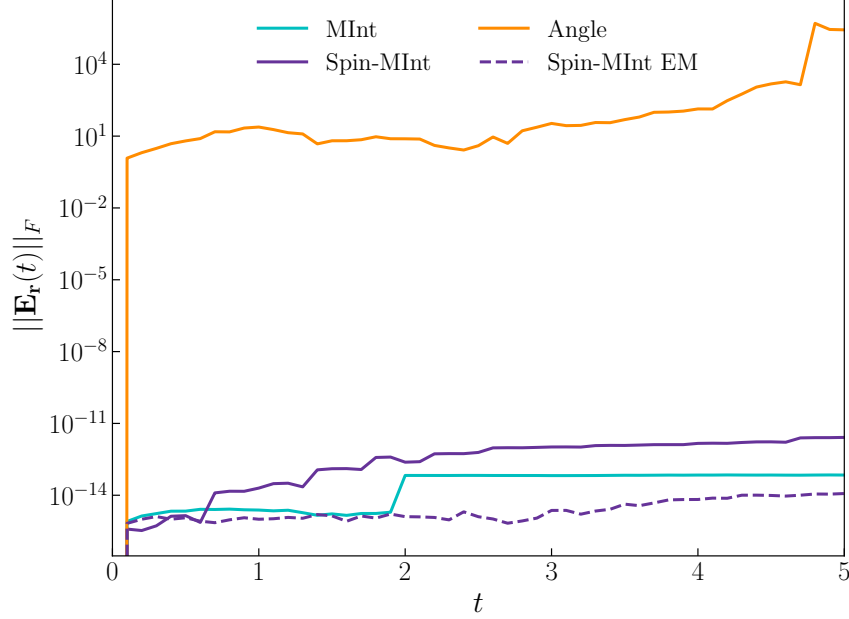

FIG. S.8. The error matrix Frobenius norm as a function of time using Model 1 for a single trajectory and  $\Delta t = 0.1$ . Here, we additionally plot the Spin-MInt explicit monodromy outlined in Section ID (dashed purple) as well as the Spin-MInt generalised monodromy from the main manuscript (purple), MInt (cyan) and angle-based (orange). We see the explicit form results in less build-up of floating point errors compared to the generalised form but is algebraically challenging to obtain for  $N > 2$ .

## B. Ensemble

### 1. Model 1

Utilising Model 1, we determine the structure preservation of the Spin-MInt algorithm. Structure preservation requires that the magnitude of the spin-vector is conserved. In Figure S.9, we plot the absolute value of the structure preservation criterion,  $|(|\mathbf{u}|(t) - |\mathbf{u}|(0))|$ , averaged over

the ensemble of trajectories using three timesteps  $\Delta t = 1.0$  (dashed),  $\Delta t = 0.1$  (solid),  $\Delta t = 0.01$  (dotted). We see that all three timesteps result in conservation of the spin-vector magnitude by noting the scale of the y-axis. The smaller timesteps appear to have poorer conservation but this is due to more opportunity of build-up of floating point errors as seen earlier in the symplecticity criterion. Hence, the Spin-MInt algorithm is structure preserving, in agreement with the theoretical prediction in the main manuscript.

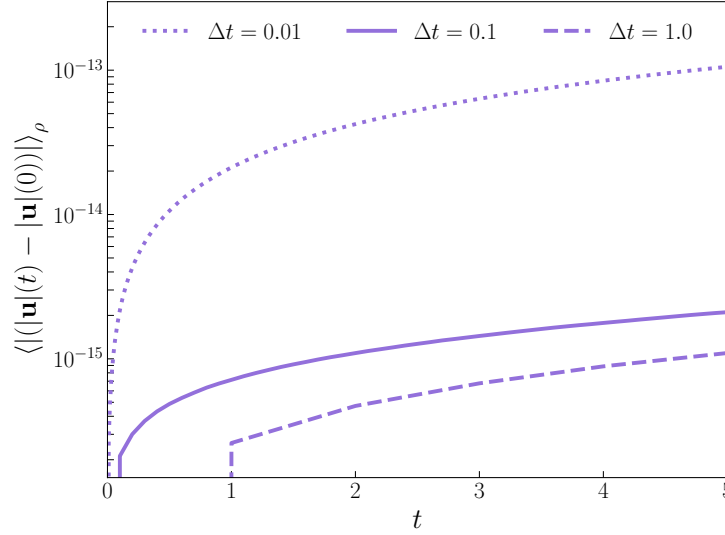

FIG. S.9. The absolute deviation in the magnitude of the spin-vector,  $\mathbf{u}$ , against time for Model 1 with an ensemble of trajectories using the Spin-MInt algorithm and three timesteps,  $\Delta t = 1.0$  (dashed),  $\Delta t = 0.1$  (solid),  $\Delta t = 0.01$  (dotted). All three timesteps preserve the spin-magnitude such that the Spin-MInt is structure preserving.

## 2. Models 2 and 3

Here, we provide additional plots for the energy conservation, Figure S.10 and S.11 using Models 2 and 3. The energy conservation confirms that the propagations are identical and that both algorithms are second-order with respect to timestep.

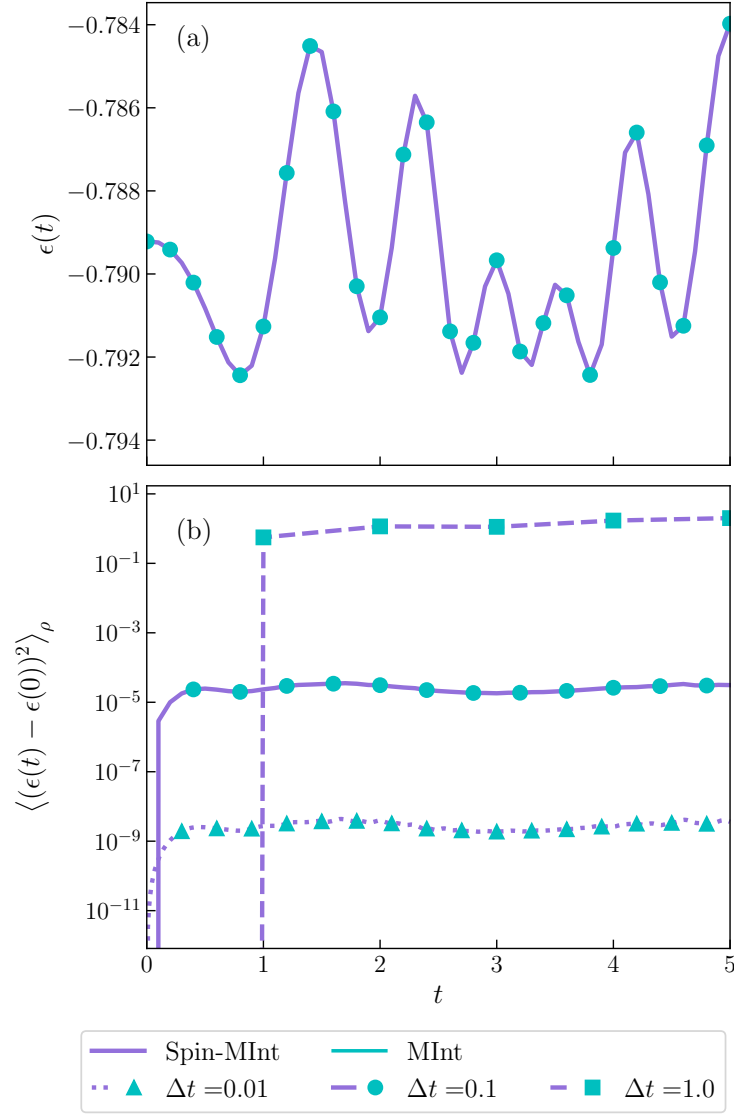

FIG. S.10. Energy conservation of Model 2 with (a) a single trajectory and  $\Delta t = 0.1$  (solid/circle) and (b) averaged using  $\Delta t = 0.1$  (solid/circle),  $\Delta t = 0.01$  (dotted/triangle) and  $\Delta t = 1.0$  (dashed/square) with the Spin-MInt (purple) and MInt (cyan) algorithms. The energies are the same for both algorithms and second-order with respect to timestep in the ensemble.

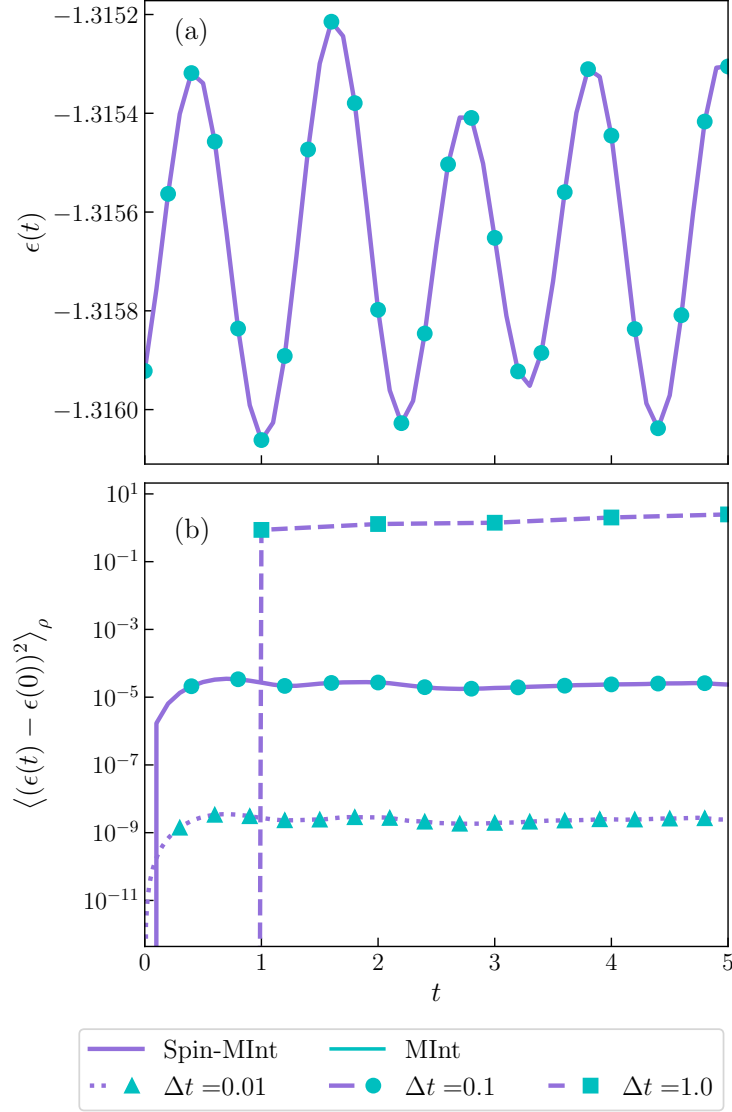

FIG. S.11. Energy conservation of Model 3 with (a) a single trajectory and  $\Delta t = 0.1$  (solid/circle) and (b) averaged using  $\Delta t = 0.1$  (solid/circle),  $\Delta t = 0.01$  (dotted/triangle) and  $\Delta t = 1.0$  (dashed/square) with the Spin-MInt (purple) and MInt (cyan) algorithms. The energies are the same for both algorithms and second-order with respect to timestep in the ensemble.

### C. Code Racing

In Table S.3, we present code racing data for the Spin-MInt and the MInt algorithms using Model 1 for the two state model and Model A for the three state model. Note that we sample MMST variables and convert into spin-mapping variables to run the Spin-MInt which may add

computational cost. For the MInt, we either leave it in MMST variables or we convert to spin-mapping variables (SM) at each timestep. This is only for comparison and we are not claiming to have the fastest implementation. The python code was run on a Standard Compute Node on Myriad at UCL and averaged over three runs.

| Algorithm                        | Two State Model      |                         | Three State Model       |
|----------------------------------|----------------------|-------------------------|-------------------------|
|                                  | With $\mathbf{M}$ /s | Without $\mathbf{M}$ /s | Without $\mathbf{M}$ /s |
| Spin-MInt                        | 829.31               | 334.96                  | 788.26                  |
| MInt ( $\mathbf{q}/\mathbf{p}$ ) | 1399.64              | 421.71                  | 566.03                  |
| MInt (SM)                        | 1439.93              | 468.26                  | 672.30                  |

TABLE S.3. Code racing results for the Spin-MInt and MInt algorithms propagating 10000 trajectories for 5 time units using  $\Delta t = 0.1$  averaged over three runs. We present two state results (Model 1), with and without monodromy matrix,  $\mathbf{M}$ , calculation and three state results (Model A). MInt ( $\mathbf{q}/\mathbf{p}$ ) remains in the MMST variables whilst MInt (SM) converts into spin-mapping variables at each timestep. For two states, the Spin-MInt is significantly faster than using the MInt. However, the Spin-MInt appears to have poorer scaling with the number of electronic states compared to the MInt.

For the two state results, we find that the Spin-MInt is approximately 40% faster than using the MInt and converting to  $\mathbf{u}$  at the end of each timestep. This becomes 30% faster when calculating the complex monodromy matrices. The MInt ( $\mathbf{q}/\mathbf{p}$ ) is only slightly faster than converting to  $\mathbf{u}$  and still much slower than the Spin-MInt. This means it is faster to use the Spin-MInt than to compute the dynamics with the MInt and transform into the spin-mapping variables at each timestep or to compute the observables directly in MMST variables for the two-level system. In comparison to previous work,<sup>9</sup> this implementation of the MInt is faster due to the alternative ordering of propagation of sub-Hamiltonians.<sup>1</sup>

However, as the electronic spin variables scale as  $N^2 - 1$ , compared to  $2N$  for the MInt, the three state model is slightly slower using the Spin-MInt. Our generalised code computes a basis set to transform between MMST and spin-mapping variables, which adds computational cost as it is utilised in the MInt (SM) but not in MInt ( $\mathbf{q}/\mathbf{p}$ ). As we sample MMST variables before converting to spin-mapping variables to propagate with the Spin-MInt, this may be adding computational cost and may be mitigated by sampling in spin-mapping variables. Additionally, computing the  $\mathbf{W}$  matrix becomes costly as this becomes very large.

Overall, the Spin-MInt is significantly faster than the MInt for a two-level system and only slightly slower for the three state model. In the case where sampling is done in spin-mapping variables, it may still be advantageous to use the Spin-MInt for  $N > 2$  due to the removal of a co-ordinate transform.

## REFERENCES

- <sup>1</sup>M. S. Church, T. J. H. Hele, G. S. Ezra, and N. Ananth, J. Chem. Phys. **148**, 102326 (2018).
- <sup>2</sup>T. J. Hele and N. Ananth, Faraday Discuss. **195**, 269 (2016).
- <sup>3</sup>L. E. Cook and T. J. H. Hele, J. Chem. Phys. **163**, 174113 (2025).
- <sup>4</sup>J. O. Richardson and M. Thoss, J. Chem. Phys. **139**, 031102 (2013).
- <sup>5</sup>J. O. Richardson, P. Meyer, M.-O. Pleinert, and M. Thoss, Chem. Phys. **482**, 124 (2017).
- <sup>6</sup>J. Tranchida, S. J. Plimpton, P. Thibaudau, and A. P. Thompson, J. Comput. Phys. **372**, 406 (2018).
- <sup>7</sup>B. Leimkuhler and S. Reich, *Simulating Hamiltonian Dynamics* (Cambridge University Press, 2005).
- <sup>8</sup>Z. Huang, H. Wang, and B. Xu, “Symplectic Spin-Lattice Dynamics with Machine-Learning Potentials,” (2025), arXiv:2506.12877 [cond-mat].
- <sup>9</sup>L. E. Cook, J. E. Runeson, J. O. Richardson, and T. J. H. Hele, J. Chem. Theory Comput. **19**, 6109 (2023).
- <sup>10</sup>D. Bossion, S. N. Chowdhury, and P. Huo, J. Chem. Phys. **154**, 184106 (2021).
- <sup>11</sup>D. Bossion, W. Ying, S. N. Chowdhury, and P. Huo, J. Chem. Phys. **157**, 084105 (2022).
- <sup>12</sup>E. A. Coronado, J. Xing, and W. H. Miller, Chem. Phys. Lett. **349**, 521 (2001).
